# Supplementary material for: VLA$^3$: Towards Native Spatial Super-Sensing in Vision Language Action Model
Source: arXiv:2611.40705 source file (2026-11-30)
Supplement: Supplementary file 1 [file appendix.tex]

\iffalse
\section{Datasets}
\subsection{Spatial understanding}
Figure~\ref{fig:3d_task fig} visualizes several cases of the spatial understanding tasks included in our evaluation, covering metric depth estimation, relative depth, and camera pose estimation. Our formulation follows previous work except for two design choices: (1) instead of resizing all images to a unified focal length to resolve camera ambiguity, we keep the native resolution and specify the horizontal and vertical field of view in the text prompt~\cite{seed1.5-vl}, an angular parameterization that is also adopted by feed-forward 3D foundation models~\cite{vggt} and is invariant to the input image size~\cite{unidepth}; (2) for absolute depth, we label the principal-axis (forward--backward) distance rather than the Euclidean distance to the camera center, i.e., the metric depth that expert vision models predict~\cite{zoedepth,unidepth}, which is interconvertible with the latter given the camera intrinsics~\cite{depthlm}.
\begin{comment}
3D/4D detection and object--camera motion prediction are constructed from simulation, relative depth sorting, and absolute depth estimation mix publicly available 3D benchmarks with pseudo-labels on real-robot data, and egomotion prediction uses simulation and public data only
\end{comment}

\subsection{Spatial grounding}
Since predictions are generated as text-based answers to sparse queries, benchmark metrics designed for dense outputs are not directly applicable. We therefore define bounded scores by averaging over all queries in each dataset. For depth, given the predicted depth $\hat d_i$ and ground truth $d_i$ for the $i$-th query, we define
\begin{equation}
    S_d=\frac{1}{N}\sum_{i=1}^{N}
    \left[
    1-\min\left(\frac{|\hat d_i-d_i|}{d_i},\,1\right)
    \right].
\end{equation}
For pose, we jointly evaluate rotation and translation:
\begin{equation}
    S_p=\frac{1}{2N}\sum_{i=1}^{N}
    \left[
        \exp\left(-\frac{e_{R,i}}{\tau_R}\right)
        +\exp\left(-\frac{e_{t,i}}{\tau_{t,i}}\right)
    \right],
    \qquad
    \tau_R=5^\circ,
    \quad
    \tau_{t,i}=\frac{\|\mathbf t_i\|_2}{5},
\end{equation}
where $e_{R,i}$ is the geodesic rotation error and
$e_{t,i}=\|\hat{\mathbf t}_i-\mathbf t_i\|_2$ is the Euclidean translation error for the $i$-th query. Here, $N$ denotes the number of queries in the corresponding dataset. An unparseable response contributes zero to the average. Both scores lie in $[0,1]$ and are reported as percentages; the ``Average'' row in Table~\ref{tab:benchmarks} reports the unweighted mean across the five datasets for each task.
%\subsection{Hello World}

\begin{figure}[t]
  \centering
  \includegraphics[width=\textwidth]{fig/appendix_spatia_understanding_fig.pdf}
  \caption{Test samples of spatial grounding.}
  \label{fig:3dtask}
\end{figure}

\subsection{Robot manipulation}
The descriptions of each robot manipulation task are provided below:
\begin{itemize}
    \item Plate stack: place the plate on the table / in the microwave / in the storage box. 
    \item Bottle upright: place the beverage bottle upright on the table.
    \item Desk trash: place the crumpled paper on the table into the trash bin.
    \item Get toast: remove the toast from the toaster.
    \item Cutlery box: place the cutlery in the storage box.
    \item Store blocks: place the building blocks in the storage box.
    \item Place blocks: take the building blocks out of the toy box and place them on the table.
    \item Cup coaster: place a cup in the center of the coaster.
    \item Refill water: place the bottle of mineral water in the storage box.
    \item Seasoning bottle: place the seasoning bottle on the spice rack.
    \item Fruit high plate: place the fruit on the table back into the elevated storage basket.
\end{itemize}
\fi
